# Supplementary material for: Rapid Neural Architecture Search by Learning to Generate Graphs from Datasets
Source: arXiv:2107.00860 source file (2021-07-02)
Supplement: Supplementary file 1 [file table_fewshot_appendix.tex]

\begin{wraptable}{r}{0.6\textwidth}
\vspace{-0.1in}
\resizebox{0.6\textwidth}{!}{
\vspace{-0.15in}

	\begin{tabular}{lc|cc}
			\hline
			\multirow{2}{*}{Method} & \multirow{2}{*}{Params (K)} & \multicolumn{2}{c}{MiniImageNet}      \\
			 &   & 5-way 1-shot & 5-way 5-shot \\
			\hline
			\hline
			MAML~\citep{finn2017model}
			& 32.9
			& 48.70
			& 63.11
			\\
	        MAML++~\citep{antoniou2018train}
			& 32.9
			& 52.15
			& 68.32
			\\
	        AutoMeta~\citep{kim2018auto}
			& 28
			& 49.58
			& 65.09
			\\
	       
	        BASE~\citep{shaw2019meta}
			& 1200
			& -
			& 66.20
			\\
			T-NAS++~\citep{lian2019towards}
			& 26.5
			& 54.11
			& 69.59
			\\
	        
	        MetaNAS~\citep{elsken2020meta}
			& 30
			& 49.7
			& 62.1
			\\
			\hline
	        MetaD2A (Ours)
			& 28.9
			& \textbf{54.71}
			& \textbf{70.59}
			\\
			\hline
		\end{tabular} 
	    }
\vspace{-0.1in}
\caption{\small {Performance on few-shot classification task}}\label{tbl:fewshot}
\vspace{-0.1in}
\end{wraptable}
