# Supplementary material for: Rapid Neural Architecture Search by Learning to Generate Graphs from Datasets
Source: arXiv:2107.00860 source file (2021-07-02)
Supplement: Supplementary file 2 [file table_predictor_appendix.tex]

\begin{wraptable}{r}{0.6\textwidth}
\vspace{-0.1in}
\resizebox{0.6\textwidth}{!}{
\vspace{-0.15in}

\begin{tabular}{cccccc}
	   % \toprule 
	   \hline
	   \multirow{2}{*}{} &
       Linear & \multirow{2}{*}{LSTM} &
       \multirow{2}{*}{GCN} &
       \multirow{2}{*}{MetaD2A-G} &
       MetaD2A-GD &
       & layer &&&& (ours)
       \\
	   \hline
	    Correlation &
	    0.0420 &
	    0.0064 &
	    0.6076 &
	    0.6426 &
	    \textbf{0.7976} \\
	    \hline
	    \end{tabular}
	    }
\vspace{-0.1in}
\caption{\small {Predictor Comparison}}\label{tbl:vae}
\vspace{-0.1in}
\end{wraptable}
